# Supplementary material for: Decentralized Detection with Signaling
Source: arXiv:1005.3062 source file (2010-05-17)
Supplement: Supplementary file 1 [file appendix.tex]

\appendices

 \section{Proof of Lemma 1}
 \begin{proof}
 Part (i) follows from definition of $\tau^1$.
 \medskip
 
 If $\tau^1 < t$, then by definition, we have 
 \begin{align} \Pi^2_t &:= P(H=0|Y^2_{1:t},U^1_{1:t}) \notag \\
 &= P(H=0|Y^2_{1:t},U^1_{1:\tau^1})
 \end{align}
 and similarly, 
 \begin{align} \Pi^2_{t+1} =  P(H=0|Y^2_{1:t+1},U^1_{1:\tau^1}), \notag  
 \end{align}
 which, on using Bayes' rule gives,
 \begin{align}
   \Pi^2_{t+1}&= \frac{P(Y^2_{t+1}|H=0)\Pi^2_t}{P(Y^2_{t+1}|H=0)\Pi^2_t + P(Y^2_{t+1}|H=1)(1-\Pi^2_t)} \label{eq:Ap1} \\
   &=: f_{t+1}(\Pi^2_{t+1},Y^2_{t+1})
 \end{align}
 Thus, we have that \[ \pi^1_{k+1} = T_k(\pi^1_k,Y^1_{k+1}), \] where \(T_k\) is defined by (\ref{eq:Ap1}).
 In Theorem 1, we defined the following value function at time \(T^1\) 
 \begin{align}
    &V_{T^1}(\pi) := min\{ \nonumber \\ &E^{\Gamma^2}[c^2\tau^2+J(U^2_{\tau^2},H)|\pi^1_{T^1}=\pi,Z^1_{1:T^1-1}=b,Z^1_{T^1}=0], \nonumber \\
                         &E^{\Gamma^2}[c^2\tau^2+J(U^2_{\tau^2},H)|\pi^1_{T^1}=\pi,Z^1_{1:T^1-1}=b,Z^1_{T^1}=1] \} \label{eq:Apb1}
 \end{align}
 Consider the first term in (\ref{eq:Apb1}). A fixed policy \(\Gamma^2\) of O2 induces a stopping time function \(S^{\Gamma^2}\) and an estimate function \(R^{\Gamma^2}\) defined for all possible realizations of the observations of O2 and messages from O1 such that
\begin{subequations}
\begin{equation}
   \tau^2 = S^{\Gamma^2}(Y^2_{1:T^2},Z^1_{1:T^1})
\end{equation}
\begin{equation}
      U^2_{\tau^2} = R^{\Gamma^2}(Y^2_{1:T^2},Z^1_{1:T^1})
\end{equation}
\end{subequations}
Using these functions in first term of (\ref{eq:Apb1}), we get
\begin{align}
 	&E^{\Gamma^2}[c^2\tau^2+J(U^2_{\tau^2},H)|\pi^1_{T^1}=\pi,Z^1_{1:T^1-1}=b,Z^1_{T^1}=0] \nonumber \\
 	= &E^{\Gamma^2}[c^2S^{\Gamma^2}(Y^2_{1:T^2},Z^1_{1:T^1}) + \nonumber \\ &J(R^{\Gamma^2}(Y^2_{1:T^2},Z^1_{1:T^1}),H)|\pi^1_{T^1}=\pi,Z^1_{1:T^1-1}=b,Z^1_{T^1}=0] \nonumber\\
 	=&E^{\Gamma^2}[c^2S^{\Gamma^2}(Y^2_{1:T^2},b_{1:T^1-1},0) +\nonumber\\
 	&J(R^{\Gamma^2}(Y^2_{1:T^2},b_{1:T^1-1},0),H)|\pi^1_{T^1}=\pi,Z^1_{1:T^1-1}=b,\nonumber \\ &Z^1_{T^1}=0]\label{eq:Apb2}
\end{align}
where we substituted \(Z^1_{1:T^1}\) in (\ref{eq:Apb2}) with the values specified in the conditioning term of the expectation. Since the only random variables left in the expectation in (\ref{eq:Apb2}) are \(Y^2_{1:T^2}\) and \(H\), we can write this expectation as
 \begin{align}
 	&\sum\limits_{\{h=0,1\}} \sum\limits_{y^2_{1:T^2} \in \mathcal{Y}^{2}_{1:T^2}} [ \nonumber \\ &P(y^2_{1:T^2},H=h|\pi^1_{T^1}=\pi,Z^1_{1:T^1-1}=b,Z^1_{T^1}=0) \nonumber \\ &\{c^2S^{\Gamma^2}(y^2_{1:T^2},b_{1:T^1-1},0) \nonumber \\&+J(R^{\Gamma^2}(y^2_{1:T^2},b_{1:T^1-1},0),h)\}] \label{eq:Apb3}
 \end{align}
 Consider first the term for \(h=0\) in (\ref{eq:Apb3}). Because of the conditional independence of the observations at the two observers, we can write this term as follows:
 \begin{align}
   &\sum\limits_{y^2_{1:T^2} \in \mathcal{Y}^{2}_{1:T^2}} [P(y^2_{1:T^2}|H=0).\pi. \nonumber \\ &\{c^2S^{\Gamma^2}(y^2_{1:T^2},b_{1:T^1-1},0)+J(R^{\Gamma^2}(y^2_{1:T^2},b_{1:T^1-1},0),0)\}] \nonumber \\
   =&\pi \times \nonumber \\ &[\sum\limits_{y^2_{1:T^2} \in \mathcal{Y}^{2}_{1:T^2}}P(y^2_{1:T^2}|H=0).\{c^2S^{\Gamma^2}(y^2_{1:T^2},b_{1:T^1-1},0) \nonumber \\ &+J(R^{\Gamma^2}(y^2_{1:T^2},b_{1:T^1-1},0),0)\}] \label{eq:Apb4} \\
   =&\pi \times A^{\Gamma^2}_{T^1} \label{eq:Apb5}
\end{align}
where \(A^{\Gamma^2}_{T^1}\) is the factor multiplying \(\pi\) in (\ref{eq:Apb4}). Note that this factor  depends only on the choice of O2's policy. Similar arguments for the term corresponding to \(h=1\) in (\ref{eq:Apb3}) show that it can be expressed as
\begin{align}
%&(1-\pi) \times [\sum\limits_{y^2_{1:T^2} \in %\mathcal{Y}^{2}_{1:T^2}}P(y^2_{1:T^2}|H=1).\{c^2S^{\Gamma^2}(y^2_{1:T^2},b_{1:T^1-1},0)+J(R^{\Gamma^2}(y^2_{1:T^2},b_{1:T^1-1},0),1)\}] \nonumber %\\
   &(1-\pi) \times B^{\Gamma^2}_{T^1} \label{eq:Apb6}
\end{align}
Equations (\ref{eq:Apb5}) and (\ref{eq:Apb6}) imply that first term of (\ref{eq:Apb1}) is a affine function of \(\pi\), given as \(A^{\Gamma^2}_{T^1}.\pi + B^{\Gamma^2}_{T^1}.(1-\pi)\). Similar arguments hold for the second term of (\ref{eq:Apb1}). Hence, we have that
\[ V_{T^1}(\pi) := min\{ L^{0}_{T^1}(\pi), L^{1}_{T^1}(\pi)\}\]
Also, since \(V_{T^1}\) is minimum of two affine functions, it is a concave function of \(\pi\). 
Now consider \(V_k\),
\begin{align}
  &V_{k}(\pi) := min\{ \nonumber \\&E^{\Gamma^2}[c^2\tau^2+J(U^2_{\tau^2},H)|\pi^1_{k}=\pi,Z^1_{1:k-1}=b,Z^1_{k}=0], \nonumber \\
                          &E^{\Gamma^2}[c^2\tau^2+J(U^2_{\tau^2},H)|\pi^1_{k}=\pi,Z^1_{1:k-1}=b,Z^1_{k}=0], \nonumber \\
                          &c^1 + E[V_{k+1}(T_k(\pi^1_k,Y^1_{k+1}))|\pi^1_{k}=\pi,Z^1_{1:k}=b]                 \} \label{eq:Apb7}
 \end{align} 
 Repeating the arguments used for \(V_{T^1}\), it can be shown that first two terms in (\ref{eq:Apb7}) are affine functions of \(\pi\). These are the functions \(L^0_k\) and \(L^1_k\) in the statement of \emph{Lemma 1} (equation \ref{eq:PFlemma1}). To prove that the third term is concave function of \(\pi\), first assume that \(V_{k+1}\) is a concave function of \(\pi\). (This is true when \(k+1=T^1\)). Then, \(V_{k+1}\) can be written as an infimum of affine functions
 \begin{equation} \label{eq:Ap1infimum}
  V_{k+1}(\pi) = \inf_i \{\lambda_i\pi + \mu_i \} \end{equation}
 The last term in (\ref{eq:Apb7}) can be written as:
 \begin{align}
 	&c^1 + E[V_{k+1}(T_k(\pi,Y^1_{k+1}))|\pi^1_{k}=\pi,Z^1_{1:k}=b] \nonumber \\
 	= &c^1 + \sum\limits_{y^1_{k+1} \in \mathcal{Y}^1} [Pr(y^1_{k+1}|\pi^1_k=\pi). V_{k+1}(T_k(\pi,y^1_{k+1})) ] 
 	\end{align}
 %Now using the characterization of \(V_{k+1}\) as infimum of affine functions and simplifying further, we get
 \begin{align}	
 	&= c^1 + \sum\limits_{y^1_{k+1} \in \mathcal{Y}^1}[\inf_i \{\lambda_i.P(y^1_{k+1}|H=0).\pi + \nonumber \\ &(Pr(y^1_{k+1}|H=0).\pi+Pr(y^1_{k+1}|H=1).(1-\pi)).\mu_i \}] \label{eq:Apb8}
 \end{align} 
 where the last equality in (\ref{eq:Apb8}) follows from (\ref{eq:Ap1}) and (\ref{eq:Ap1infimum}).
 Observe that the expression within the infimum is an affine function of \(\pi\). Hence, taking the infimum over \(i\) gives a concave function of \(\pi\) for each \(y^1_{k+1}\). Since the sum of concave functions is concave, we have that the expression in (\ref{eq:Apb8}) is a concave function of \(\pi\). We call this function \(G_k(\pi)\). Thus, the value function at time \(k\) can be expressed as:
  \begin{equation}
  V_{k}(\pi) := min\{ L^{0}_k(\pi), L^{1}_k(\pi), G_k(\pi)\} \label{eq:Apb9}
  \end{equation}
  Since \(V_k\) is minimum of a concave and two affine functions, it itself is a concave function. This completes the argument for induction and (\ref{eq:Apb9}) now holds for all \(k=(T^1-1),...,2,1\).  
 \end{IEEEproof}
